# Supplementary material for: Ferro-Orbital Order and Strong Magnetic Anisotropy in the Parent Compounds of Iron-Pnictide Superconductors
Source: arXiv:0905.2957 source file (2009-12-08)
Supplement: Supplementary file 1 [file Supplementary.pdf]

[Supplementary Information] **Ferro-Orbital Order and Strong Magnetic Anisotropy in the Parent Compounds of Iron-Pnictide Superconductors**

Chi-Cheng Lee, Wei-Guo Yin, and Wei Ku

## Topic A: Detecting the same orbital ordering for different Wannier function decompositions

There exists a gauge freedom in the Wannier Function (WF) construction [19]. While the physics of orbital ordering is independent of a particular setup, its manifestations could be different for different setups. Among them, the most convenient (intuitive) is the one that gives rise to the diagonal representation of the local (on-site) one-particle density matrix, $\rho$.

In the present WF construction, the coordinate system is rotated 45° about the z axis compared to the previous studies [9,20] that employed the maximally localized Wannier functions (MLWFs) [19]. These two sets of WF decompositions are approximately related via the following local electron annihilation operators:

$$d_{xz} = \frac{1}{\sqrt{2}}(D_{XZ} + D_{YZ}),$$
$$d_{yz} = \frac{1}{\sqrt{2}}(D_{XZ} - D_{YZ}),$$

where $d_{xz}$ and $d_{yz}$ are for our WFs, while $D_{XZ}$ and $D_{YZ}$ are for previous MLWFs. Note that strictly speaking, such post-process mixture of MLWFs delocalizes slightly the WFs in comparison to our direct symmetry-respecting construction. Nevertheless, we find that they are essentially the same by comparing the electron hopping integrals in the same coordinate system.

Using our setup (the x and y directions are chosen to point to the first-neighbor Fe atoms), we find, as shown in Table S1, that $\rho$ is always diagonalized in the Fe $3d_{xz}$ and $3d_{yz}$ subspace no matter whether the orbital ordering exists or not, namely

$$\rho = \begin{pmatrix} \langle d^{\dagger}_{xz} d_{xz} \rangle & \langle d^{\dagger}_{xz} d_{yz} \rangle \\ \langle d^{\dagger}_{yz} d_{xz} \rangle & \langle d^{\dagger}_{yz} d_{yz} \rangle \end{pmatrix} = \begin{pmatrix} \langle d^{\dagger}_{xz} d_{xz} \rangle & 0 \\ 0 & \langle d^{\dagger}_{yz} d_{yz} \rangle \end{pmatrix}.$$

Therefore, the orbital polarization and ordering are manifested directly via the imbalanced occupation numbers $\langle d^{\dagger}_{xz} d_{xz} \rangle$ and $\langle d^{\dagger}_{yz} d_{yz} \rangle$.

Whereas, using the setup for those MLWFs (the X and Y directions are chosen to point to the second-neighbor Fe atoms),

$$\rho = \begin{pmatrix} \langle D^{\dagger}_{XZ} D_{XZ} \rangle & \langle D^{\dagger}_{XZ} D_{YZ} \rangle \\ \langle D^{\dagger}_{YZ} D_{XZ} \rangle & \langle D^{\dagger}_{YZ} D_{YZ} \rangle \end{pmatrix} = \frac{1}{2} \begin{pmatrix} \langle d^{\dagger}_{xz} d_{xz} \rangle + \langle d^{\dagger}_{yz} d_{yz} \rangle & \langle d^{\dagger}_{xz} d_{xz} \rangle - \langle d^{\dagger}_{yz} d_{yz} \rangle \\ \langle d^{\dagger}_{xz} d_{xz} \rangle - \langle d^{\dagger}_{yz} d_{yz} \rangle & \langle d^{\dagger}_{xz} d_{xz} \rangle + \langle d^{\dagger}_{yz} d_{yz} \rangle \end{pmatrix}.$$

It becomes clear that the occupation numbers of the XZ and YZ orbitals are always the same. In this case, **to determine whether the orbital ordering exists, one has to check if the off-diagonal terms $\left\langle D^{\dagger}_{XZ} D_{YZ} \right\rangle$ and $\left\langle D^{\dagger}_{YZ} D_{XZ} \right\rangle$ are finite.** This is the so-called spontaneous hybridization, since by symmetry the on-site off-diagonal terms are zero in the normal state. This important point could be easily overlooked, since computation of the off-diagonal elements of $\rho$ in the Wannier basis is not as a common practice as the diagonal ones.

$\rho$'s of LDA, LSDA and LSDA+U calculations in the two different WF decompositions are listed in Table S1. The LDA results indicate that for the nonmagnetic case both WF decompositions give the diagonal representation of $\rho$. Thus, it is confirmed that the local xz-yz or XZ-YZ hybridization is indeed prohibited by symmetry in the normal state. On the other hand, the spin-polarized calculations confirm the above analysis: the orbital order manifests itself clearly as imbalanced occupations in the present work, while it hides as spontaneous hybridization in previous studies based on MLWF.

Table S1: Local one-particle density matrix in two Fe 3*d* Wannier basis sets.

(a) The x and y directions are chosen to point to the first-neighbor Fe atoms

LDA

| | $z^2$ | $x^2$-$y^2$ | yz | xz | xy |
|---|---|---|---|---|---|
| $z^2$ | 0.685 | 0.000 | 0.000 | 0.000 | 0.000 |
| $x^2$-$y^2$ | 0.000 | 0.519 | 0.000 | 0.000 | 0.000 |
| yz | 0.000 | 0.000 | 0.631 | 0.000 | 0.000 |
| xz | 0.000 | 0.000 | 0.000 | 0.631 | 0.000 |
| xy | 0.000 | 0.000 | 0.000 | 0.000 | 0.512 |

LSDA

| Spin up | $z^2$ | $x^2$-$y^2$ | yz | xz | xy |
|---|---|---|---|---|---|
| $z^2$ | 0.811 | -0.025 | 0.000 | 0.000 | 0.000 |
| $x^2$-$y^2$ | -0.025 | 0.655 | 0.000 | 0.000 | 0.000 |
| yz | 0.000 | 0.000 | 0.749 | 0.000 | 0.000 |
| xz | 0.000 | 0.000 | 0.000 | 0.725 | 0.000 |
| xy | 0.000 | 0.000 | 0.000 | 0.000 | 0.614 |
| Spin down | $z^2$ | $x^2$-$y^2$ | yz | xz | xy |
| $z^2$ | 0.556 | 0.066 | 0.000 | 0.000 | 0.000 |
| $x^2$-$y^2$ | 0.066 | 0.463 | 0.000 | 0.000 | 0.000 |
| yz | 0.000 | 0.000 | 0.411 | 0.000 | 0.000 |
| xz | 0.000 | 0.000 | 0.000 | 0.576 | 0.000 |
| xy | 0.000 | 0.000 | 0.000 | 0.000 | 0.355 |

LSDA+U (U=2eV, J=0.5eV)

| Spin up | $z^2$ | $x^2$-$y^2$ | yz | xz | xy |
|---|---|---|---|---|---|
| $z^2$ | 0.890 | -0.010 | 0.000 | 0.000 | 0.000 |
| $x^2$-$y^2$ | -0.010 | 0.859 | 0.000 | 0.000 | 0.000 |
| yz | 0.000 | 0.000 | 0.819 | 0.000 | 0.000 |
| xz | 0.000 | 0.000 | 0.000 | 0.849 | 0.000 |
| xy | 0.000 | 0.000 | 0.000 | 0.000 | 0.744 |
| Spin down | $z^2$ | $x^2$-$y^2$ | yz | xz | xy |
| $z^2$ | 0.316 | 0.167 | 0.000 | 0.000 | 0.000 |
| $x^2$-$y^2$ | 0.167 | 0.386 | 0.000 | 0.000 | 0.000 |
| yz | 0.000 | 0.000 | 0.243 | 0.000 | 0.000 |
| xz | 0.000 | 0.000 | 0.000 | 0.615 | 0.000 |
| xy | 0.000 | 0.000 | 0.000 | 0.000 | 0.226 |

(b) The X and Y directions are chosen to point to the second-neighbor Fe atoms

LDA

| | $Z^2$ | $X^2$-$Y^2$ | YZ | XZ | XY |
|---|---|---|---|---|---|
| $Z^2$ | 0.685 | 0.000 | 0.000 | 0.000 | 0.000 |
| $X^2$-$Y^2$ | 0.000 | 0.512 | 0.000 | 0.000 | 0.000 |
| YZ | 0.000 | 0.000 | 0.631 | 0.000 | 0.000 |
| XZ | 0.000 | 0.000 | 0.000 | 0.631 | 0.000 |
| XY | 0.000 | 0.000 | 0.000 | 0.000 | 0.519 |

LSDA

| Spin up | $Z^2$ | $X^2$-$Y^2$ | YZ | XZ | XY |
|---|---|---|---|---|---|
| $Z^2$ | 0.811 | 0.000 | 0.000 | 0.000 | -0.025 |
| $X^2$-$Y^2$ | 0.000 | 0.614 | 0.000 | 0.000 | 0.000 |
| YZ | 0.000 | 0.000 | 0.737 | -0.012 | 0.000 |
| XZ | 0.000 | 0.000 | -0.012 | 0.737 | 0.000 |
| XY | -0.025 | 0.000 | 0.000 | 0.000 | 0.655 |
| Spin down | $Z^2$ | $X^2$-$Y^2$ | YZ | XZ | XY |
| $Z^2$ | 0.556 | 0.000 | 0.000 | 0.000 | 0.066 |
| $X^2$-$Y^2$ | 0.000 | 0.355 | 0.000 | 0.000 | 0.000 |
| YZ | 0.000 | 0.000 | 0.494 | 0.082 | 0.000 |
| XZ | 0.000 | 0.000 | 0.082 | 0.494 | 0.000 |
| XY | 0.066 | 0.000 | 0.000 | 0.000 | 0.463 |

LSDA+U (U=2eV, J=0.5eV)

| Spin up | $Z^2$ | $X^2$-$Y^2$ | YZ | XZ | XY |
|---|---|---|---|---|---|
| $Z^2$ | 0.890 | 0.000 | 0.000 | 0.000 | -0.010 |
| $X^2$-$Y^2$ | 0.000 | 0.744 | 0.000 | 0.000 | 0.000 |
| YZ | 0.000 | 0.000 | 0.834 | 0.015 | 0.000 |
| XZ | 0.000 | 0.000 | 0.015 | 0.834 | 0.000 |
| XY | -0.010 | 0.000 | 0.000 | 0.000 | 0.859 |

| Spin down | $Z^2$ | $X^2$-$Y^2$ | YZ | XZ | XY |
|---|---|---|---|---|---|
| $Z^2$ | 0.316 | 0.000 | 0.000 | 0.000 | 0.167 |
| $X^2$-$Y^2$ | 0.000 | 0.226 | 0.000 | 0.000 | 0.000 |
| YZ | 0.000 | 0.000 | 0.429 | 0.186 | 0.000 |
| XZ | 0.000 | 0.000 | 0.186 | 0.429 | 0.000 |
| XY | 0.167 | 0.000 | 0.000 | 0.000 | 0.386 |

## Topic B: Visualizing the unconventional $d_{xz}$-$d_{xz}$ and $d_{yz}$-$d_{yz}$ hopping integrals between the Wannier orbitals

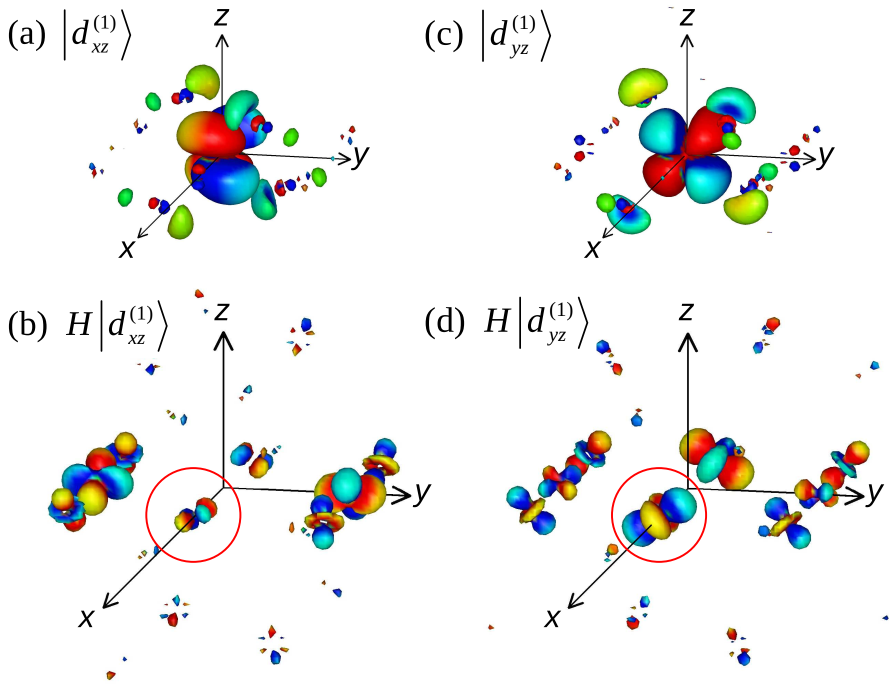


Figure S1: (a) The real-space picture of $\left|d_{xz}^{(1)}\right\rangle$, the $3d_{xz}$ Wannier orbital of an iron atom (referred to as Fe1). (b) The wave function obtained from applying the Kohn-Sham Hamiltonian, $H$, to the Fe1 $3d_{xz}$ orbital. The small portion on Fe2 (the nearest-neighbor Fe atom of Fe1 along the $x$ direction) is highlighted by a red circle. (c) and (d) are the counterpart for the Fe1 $3d_{yz}$ Wannier orbital ($\left|d_{yz}^{(1)}\right\rangle$ and $H\left|d_{yz}^{(1)}\right\rangle$, respectively). The surprisingly large portion of $H\left|d_{yz}^{(1)}\right\rangle$ on Fe2, as highlighted by a red circle in (d), is oriented along the direction facilitating a substantially large overlap with the Fe2 $3d_{yz}$ orbital.

Consider

$t^{x}_{xz,xz} = \langle d^{(2)}_{xz} | H | d^{(1)}_{xz} \rangle$,

$t^{x}_{yz,yz} = \langle d^{(2)}_{yz} | H | d^{(1)}_{yz} \rangle$,

where $|d^{(i)}_{xz}\rangle$ and $|d^{(i)}_{yz}\rangle$ are the $3d_{xz}$ and $3d_{yz}$ Wannier orbitals on the *i*-th Fe atom; the first (Fe1) and the second (Fe2) iron atoms are the nearest neighbors (NN) along the *x* axis. *H* is the Kohn-Sham Hamiltonian of the first-principles band structure calculations.

The Wannier functions (WF) of $|d^{(1)}_{xz}\rangle$ and $H|d^{(1)}_{xz}\rangle$ are shown in Fig. S1(a) and S1(b), respectively. The magnitude of $t^{x}_{xz,xz}$ (i.e., the overlap between $H|d^{(1)}_{xz}\rangle$ and $|d^{(2)}_{xz}\rangle$ — the WF of $|d^{(2)}_{xz}\rangle$ is just the translation of the WF of $|d^{(1)}_{xz}\rangle$ from Fe1 to Fe2 with a reflection on xz plane) is mainly determined by the overlap of the portion of $H|d^{(1)}_{xz}\rangle$ on the Fe2 site, as highlighted with a circle in Fig. S1(b), and the center piece of $|d^{(1)}_{xz}\rangle$ translated to the Fe2 site. It can be easily visualized that the overlap is small, indeed.

The Wannier functions (WF) of $|d^{(1)}_{yz}\rangle$ and $H|d^{(1)}_{yz}\rangle$ are shown in Fig. S1(c) and S1(d), respectively. The magnitude of $t^{x}_{yz,yz}$ (i.e., the overlap between $H|d^{(1)}_{yz}\rangle$ and $|d^{(2)}_{yz}\rangle$ — the WF of $|d^{(2)}_{yz}\rangle$ is just the translation of the WF of $|d^{(1)}_{yz}\rangle$ from Fe1 to Fe2 with a reflection on yz plane) is mainly determined by the overlap of the portion of $H|d^{(1)}_{yz}\rangle$ on the Fe2 site, as highlighted with a circle in Fig. S1(d), and the center piece of $|d^{(1)}_{yz}\rangle$ translated to the Fe2 site. It can be easily visualized that the overlap is large, indeed.

These results are anti-intuitive: The supposedly strong "$\sigma$-bond" NN $d_{xz}$-$d_{xz}$ hopping along the *x* direction is remarkably weak, while the supposedly weak "$\pi$-bond" NN $d_{yz}$-$d_{yz}$ hopping along the *x* direction is remarkably strong. Physically, this reflects the dramatic influence of the tetrahedral positioning of As 4*p* orbitals on the low-energy physics of Fe 3*d* orbitals. As highlighted with a circle in Fig. S1(d), the portion of $H|d^{(1)}_{yz}\rangle$ on the Fe2 site is not only considerably large but also oriented toward the local yz direction due to the hybridization with the two neighboring As atoms that are located in the local yz direction. This orientation gives rise to the large overlap of $H|d^{(1)}_{yz}\rangle$ and $|d^{(2)}_{yz}\rangle$, and thus strong $t^{x}_{yz,yz}$. Such positioning of the As atoms, on the other hand, can not satisfy $t^{x}_{xz,xz}$ at the same time, leading to weak $t^{x}_{xz,xz}$.

## Topic C: Comparing energy between ferro and staggered orbital structures with the stripy antiferromagnetic order with a three-band consideration

The physics in LaOFeAs at the energy scale of about 3 eV near the Fermi level may be sufficiently described by *the multiorbital Hubbard model* with hopping integrals $t_{ij}^{\alpha\beta}$, onsite intraorbital Coulomb repulsion $U$ (about 1-3 eV), onsite interorbital Coulomb repulsion $U'$, and Hund's coupling $J$. On the other hand, to understand the magnetic and structural transitions at about 150 K (about 12 meV) and the superconducting transition below 60 K, it is desirable to start with an effective lower-energy Hamiltonian, $H_{\text{eff}}$, reduced from the Hubbard model, such that even the low-order solution of $H_{\text{eff}}$ could yield meaningful insights. The superexchange processes discussed in the manuscript result from this reduction.

In the text (Fig. 4b and Fig. 4c), we have shown that the orbital polarization on the Fe $3d_{xz}$ and $3d_{yz}$ orbitals makes the superexchange path very directional, because the nearest-neighbor hopping between the half-filled $d_{yz}$ orbitals along the $x$ direction is substantially larger than along the $y$ direction. This was demonstrated with a *two-orbital* consideration. Here we demonstrate that the directional superexchange is further enhanced via the inclusion of additional $d$-orbitals, using $3d_{x^2-y^2}$ orbital as an example from which the electrons hop to $d_{yz}$ ($d_{xz}$) along the $x$ ($y$) direction with the largest magnitude (c.f., Table I). With the *three-band* consideration, following the two leading hopping integrals found in the iron plane, we compare the superexchange energy gain between ferro-orbital and staggered orbital structures with the same stripy antiferromagnetic environment in second-order perturbation theory. (The ferromagnetic configuration suffers from reduction of AF super-exchange paths and is thus not considered here.) These two orbital orderings are illustrated in Fig. S2.

Consider

$$\Delta = \varepsilon_{xz} - \varepsilon_{x^2-y^2} = \varepsilon_{yz} - \varepsilon_{x^2-y^2},$$
$$t = \left\langle d_{yz}^{(2)} \middle| H \middle| d_{yz}^{(1)} \right\rangle = \left\langle d_{xz}^{(4)} \middle| H \middle| d_{xz}^{(1)} \right\rangle,$$
$$t' = \left\langle d_{x^2-y^2}^{(2)} \middle| H \middle| d_{yz}^{(1)} \right\rangle = \left\langle d_{x^2-y^2}^{(4)} \middle| H \middle| d_{xz}^{(1)} \right\rangle,$$

where $\left| d_{xz}^{(i)} \right\rangle$, $\left| d_{yz}^{(i)} \right\rangle$, and $\left| d_{x^2-y^2}^{(i)} \right\rangle$ are the $3d_{xz}$, $3d_{yz}$, and $3d_{x^2-y^2}$ Wannier orbitals on the $i$-th Fe atom, respectively. The leading hopping integrals among Fe $3d$ Wannier orbitals, e.g. $\left\langle d_{yz}^{(2)} \middle| H \middle| d_{yz}^{(1)} \right\rangle$ and $\left\langle d_{x^2-y^2}^{(2)} \middle| H \middle| d_{yz}^{(1)} \right\rangle$, are labeled by $t$ and $t'$. As shown in Fig. S2, the first (Fe1) and the second (Fe2) iron atoms are the nearest neighbors (NN) along the $x$ axis. The fourth (Fe4) iron atom is the nearest neighbor along the $y$ axis. $H$ is the Kohn-Sham Hamiltonian of the first-principles band structure calculations. The difference of on-site energies of $3d_{xz}$ (or $3d_{yz}$) and $3d_{x^2-y^2}$ is labeled by $\Delta$.

The energy gain per site for ferro-orbital ordering ( $\Delta E_f$ ) is

$$\Delta E_f = -\frac{2t^2}{U+J_H} - \frac{2t'^2}{\Delta+U+J_H} - \frac{2t'^2}{-\Delta+U+J_H} - \frac{2t'^2}{-\Delta+U'-J_H},$$

where $U$, $U'$, and $J_H$ denote the intra orbital Coulomb repulsion, inter orbital repulsion, and Hund's exchange, respectively. The energy gain per site for staggered orbital ordering ( $\Delta E_s$ ) is

$$\Delta E_s = -\frac{t^2}{U'-J_H} - \frac{t^2}{U'+J_H} - \frac{t'^2}{-\Delta+U+J_H} - \frac{t'^2}{\Delta+U+J_H} - \frac{t'^2}{-\Delta+U'+J_H} - \frac{t'^2}{-\Delta+U'-J_H},$$

To compare $\Delta E_f$ and $\Delta E_s$, neglecting small $J_H$ and the small difference between $U$ and $U'$, one finds that the ferro-orbital ordering gains the superexchange energy by $O(2t'^2/U)$. That is, the ferro-orbital order is lower in energy than the staggered orbital order within the same stripy magnetic configuration.

It should be made clear that the above estimation from the second-order perturbation is very crude for the Fe-pnictides, since they are metallic even without doping (implying $U/t$ not too large). Thus, screening from higher-order terms [c.f., R. Coldea et al., Phys. Rev. Lett. 86, 5377 (2001)] and charge fluctuation are in principle necessary to be taken into account. The authors of the present manuscript have recently developed a first-principles Wannier-function based numerical canonical transformation approach to the effective low-energy Hamiltonian for the cuprates [W.-G. Yin and W. Ku, Phys. Rev. B 79, 214512 (2009)]. The application and extension of this approach to Fe-pnictides is in progress.

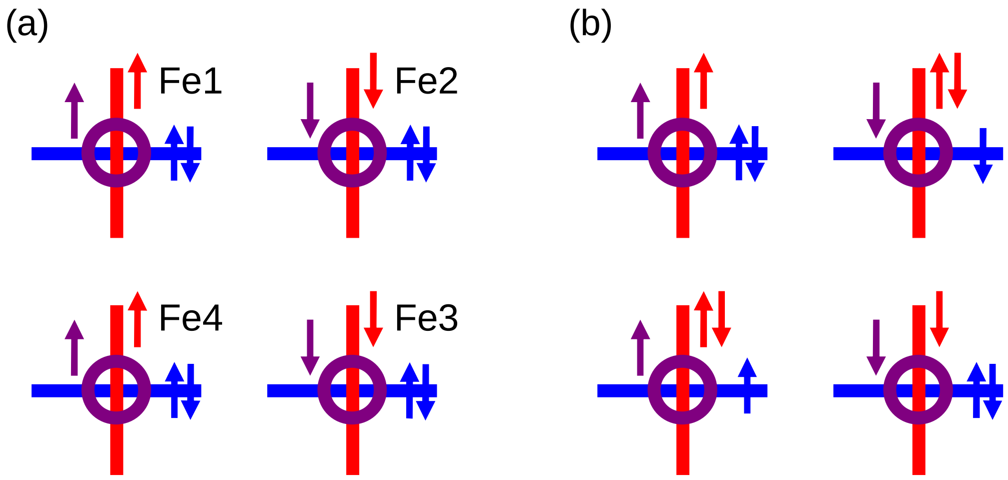


Figure S2: Illustration of (a) ferro-orbital and (b) staggered orbital structures for a 3-band consideration. The Fe $3d_{xz}$ and $3d_{yz}$ Wannier orbitals are denoted by blue and red lines, respectively. The Fe $3d_{x^2-y^2}$ orbital is presented by the purple circles. The high-spin

configuration is indicated by the arrows with the same color scheme as the corresponding Wannier orbitals.
